# Supplementary material for: Active Sampling for Accelerated MRI with Low-Rank Tensors
Source: arXiv:2012.12496 source file (2021-05-22)
Supplement: Supplementary file 1 [file appendix.tex]

%\appendix
\appendices
%\section{Subproblems in the alternating algorithms}
\section{Sub-Problems in the Block Coordinate Descent Solver}
\label{sec:appendix_BCD}
When we employ a block coordinate descent solver, \ie~solving Eq.~\reff{eq:BCD_Obj}, the decomposed subproblems are as follows:
\begin{itemize}[leftmargin=*]
\item Sub-${\mat{L}_i}$ problem: we fix $\ten{S}$ and $\ten{M}$, and then update $\{ \mat{L}_i\}$ by solving:
\begin{equation}
\label{eq:sub-L}
\begin{array}{ll}
\mathop {\min } \limits_{\{\mat{L}_i\}} & \sum\limits_{i = 1}^n {{\alpha_i}{{\left\| {{\mat{L}_i}} \right\|}_*}}  + \frac{{{\lambda_i}}}{2}\left\| {{\mat{L}_i} + {\mat{S}_{(i)}} - {\mat{M}_{(i)}}} \right\|_F^2 \\
& \equiv \sum\limits_{i = 1}^n \frac{1}{2}\left\| {{\mat{L}_i} + {\mat{S}_{(i)}} - {\mat{M}_{(i)}}} \right\|_F^2 + \frac{{{\alpha_i}}}{{{\lambda_i}}}{\left\| {{\mat{L}_i}} \right\|_*}.
\end{array}
\end{equation} 
\item Sub-$\ten{S}$ problem: we fix $\{ \mat{L}_i\}_{i=1}^n$ and $\ten{M}$, and then update $\ten{S}$ by solving:
\begin{equation}
\label{eq:sub-S}
\begin{array}{ll}
\mathop {\min }\limits_{\ten{S}} & \sum\limits_{i = 1}^n \frac{{{\lambda_i}}}{2}\left\| {{\mat{L}_i} + {\mat{S}_{(i)}} - {\mat{M}_{(i)}}} \right\|_F^2 + {\lambda}{\left\| {\mathbb{T}{\mathbb{F}^{-1}}\ten{S}} \right\|_1}\\
\end{array}
\end{equation}
\item Sub-$\ten{M}$ problem: we fix $\{ \mat{L}_i\}_{i=1}^n$ and $\ten{S}$, and then update $\ten{M}$ by solving:
\begin{equation}
\label{eq:sub-M}
\begin{aligned}
 \mathop {\min }\limits_\ten{M} \quad & \sum\limits_{i = 1}^n {\frac{{{\lambda_i}}}{2}\left\| {{\mat{L}_i} + {\mat{S}_{(i)}} - {\mat{M}_{(i)}}} \right\|_F^2}\\
  \st \quad & {\ten{M}_\Omega } = {\ten{T}_\Omega }. 
\end{aligned}
\end{equation}
\end{itemize}

\section{Sub-Problems in the Alternating direction method of multipliers (ADMM) solver}
\label{sec:appendix_admm}
Similarly, the sub-problems of ADMM, \ie~solving Eq.~\reff{eq:admm_Obj}, are shown as follows.
\begin{itemize}[leftmargin=*]
\item Sub-${\mat{L}_i}$ problem: 
\begin{equation}
\label{eq:sub-L_admm}
\begin{aligned}
\mathop{\min}\limit_{\mat{L}_i} \quad&
{\alpha_i}{{\left\| {{\mat{L}_i}} \right\|}_* } 
+ \langle \ten{M} - \text{Fold}_i({\mat{L}_i}) - \ten{S}, {\ten{Y}_i} \rangle \\
& + \frac{\rho}{2}\left\| {{\mat{L}_i} + {\mat{S}_{(i)}} - {\mat{M}_{(i)}}} \right\|_F^2. 
\end{aligned}
\end{equation}
\item Sub-$\ten{S}$ problem: 
\begin{equation}
\label{eq:sub-S_admm}
\begin{aligned}
 \mathop{\min}\limit_{\ten{S}}  \quad& {\lambda}{\left\| \mathbb{T}{\mathbb{F}^{-1}}S \right\|_1}
+ \sum\limits_{i = 1}^n \langle \ten{M} - \text{Fold}_i({\mat{L}_i}) - \ten{S}, {\ten{Y}_i} \rangle\\
& + \frac{\rho}{2}\left\| {{\mat{L}_i} + {\mat{S}_{(i)}} - {\mat{M}_{(i)}}} \right\|_F^2  
\end{aligned}
\end{equation}
\item Sub-$\ten{M}$ problem: 
\begin{equation}
\label{eq:sub-M_admm}
\begin{aligned}
  \mathop{\min}\limit_{\ten{M}} \quad & \sum\limits_{i = 1}^n \frac{\rho}{2}\left\| {{\mat{L}_i} + {\mat{S}_{(i)}} - {\mat{M}_{(i)}}} \right\|_F^2
    + \langle \ten{M} - \text{Fold}_i({\mat{L}_i}) - \ten{S}, {\ten{Y}_i} \rangle\\
    \st \quad & \ten{M}_{\Omega} = \ten{T}_{\Omega} 
\end{aligned}
\end{equation}
\item Sub-$\ten{Y}_i$ problem: 
\begin{equation}
\mathop{\min}\limit_{\ten{Y}_i} \quad  \langle \ten{M} - \text{Fold}_i({\mat{L}_i}) - \ten{S}, {\ten{Y}_i} \rangle
\end{equation}    
\end{itemize}
